# Supplementary material for: Rician likelihood loss for quantitative MRI using self-supervised deep learning
Source: arXiv:2307.07072 source file (2023-07-13)
Supplement: Supplementary file 1 [file Supp_RicianLossSSqMRIParker.pdf]

## SUPPORTING INFORMATION

|                        | $I_0(x)$                                                                                                                       | $\log(I_0(x))$                                                                                                                                                      |
|------------------------|--------------------------------------------------------------------------------------------------------------------------------|---------------------------------------------------------------------------------------------------------------------------------------------------------------------|
| Series <sup>20</sup>   | $\sum_{k=0}^{50} \frac{1}{4} \frac{(x^2)^k}{(k!)^2}$                                                                           | $\log\left(\sum_{k=0}^{50} \exp(-k\log(4) + 2k\log(x)) - 2\log\Gamma(k+1)\right)$                                                                                   |
| Hankel-1 <sup>23</sup> | $\frac{e^x}{\sqrt{2\pi x}}$                                                                                                    | $x - \frac{\log(2\pi x)}{2}$                                                                                                                                        |
| Hankel-2 <sup>24</sup> | $e^x$                                                                                                                          | $x$                                                                                                                                                                 |
| Proposed <sup>28</sup> | $e^x \sum_{i=0}^{30} c_i^{(l)} T_i(x_t), x = [0,8]$ $\frac{e^x}{\sqrt{x}} \sum_{i=0}^{25} c_i^{(h)} T_i(x_t), x = (8, \infty)$ | $x + \log\left(\sum_{i=0}^{30} c_i^{(l)} T_i(x_t)\right), x = [0,8]$ $x + \log\left(\sum_{i=0}^{25} c_i^{(l)} T_i(x_t)\right) - \frac{\log(x)}{2}, x = (8, \infty)$ |

**TABLE S1.** Approximate modified Bessel functions of the first kind with order zero and their logarithms.  $T_i(x_t)$  are Chebyshev polynomials of the first kind evaluated at  $x$  transformed to the range  $[-1,1]$  and  $c_i^*$  are vectors of coefficients for the low or high ranges of  $x$ .

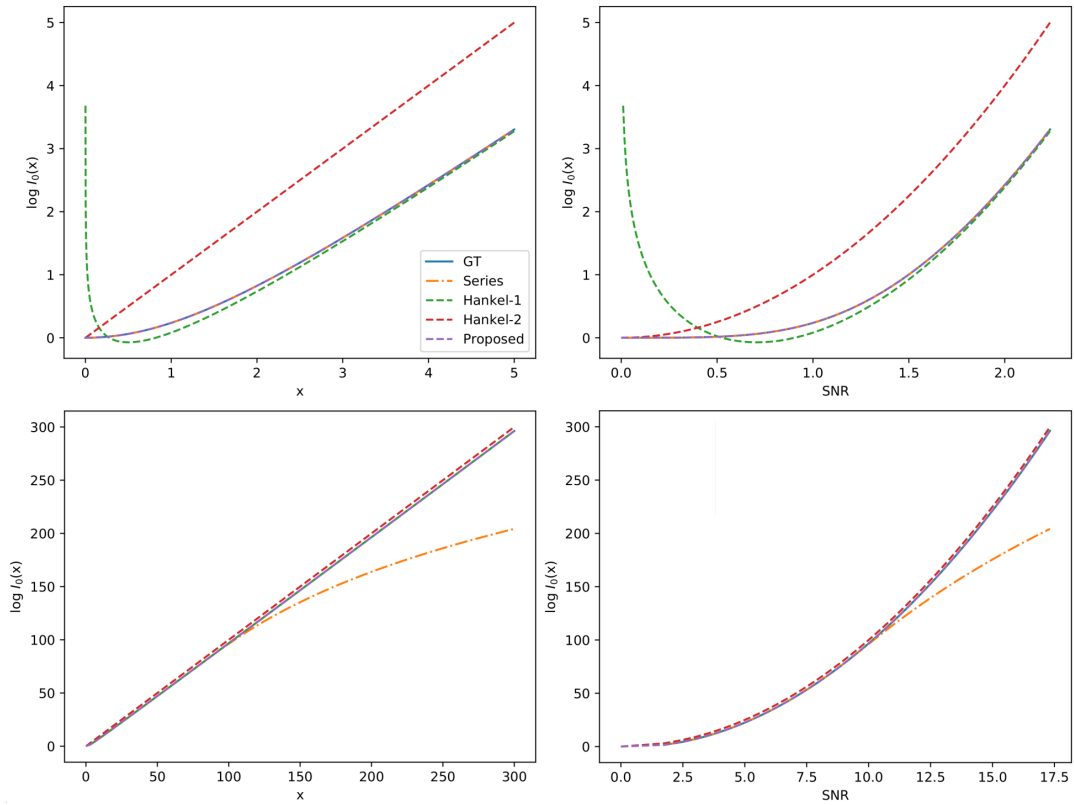

**FIGURE S1.**  $\log(I_0(x))$  approximations as a function of input,  $x$ , and  $\text{SNR} \approx \sqrt{x}$ . In the left column, plots are a function of  $x$ . In the right column, plots are a function of SNR. The top and bottom rows show different ranges of SNRs - low and high, respectively. The ground truth (GT, blue line) was computed using 1000 summations of the series expansion, which converges in value for the range of  $x$  shown. Note the GT line is only partially visible as it overlaps with the approximations. In the bottom left plot (high SNR as a function of  $x$ ), it is fully obscured by the Proposed and Hankel-1 lines.

|          | Stable training SNRs |
|----------|----------------------|
| Series   | [5, 40]              |
| Hankel-1 | [10, 40]             |
| Hankel-2 | (0, 40]              |
| Proposed | (0,40]               |

**TABLE S2.** Range of training data SNRs over which the loss functions incorporating the  $\log(I_0(x))$  approximations were numerically stable. Networks were trained on data with SNRs of (0, 40] in increments of 2.5. Training was stable if the loss function did not underflow or overflow. Proposed and Hankel-2 were stable across the entire SNR range, whereas Series and Hankel-1 were unstable at low SNR.
